# Supplementary material for: Optimized Cranial Bandeau Remodeling
Source: arXiv:1912.10601 source file (2021-03-13)
Supplement: Supplementary file 1 [file appendix.tex]

\section{Omitted Proofs}\label{appendix:proofs}
